# Supplementary material for: Leveraging Experience in Lazy Search
Source: arXiv:1907.07238 source file (2019-07-16)
Supplement: Supplementary file 1 [file appendix.tex]

% !TEX root = ../main.tex

\appendices

\section{}
\label{appendix:bern}

We will show here that if $P(\world)$ is an independent Bernoulli distribution over edges $\vectorp$ and no two paths $\path_i, \path_j$ share an edge, the optimal \selector is the one that picks the edge on the shortest path with the lowest probability. Intuitively, the selector tries to eliminate each path as quickly as possible - the lack of overlap implies the selector does not have to reason over the consequences of eliminating a path.

We first define a selector \selectorFailFast:
\begin{equation}
	\selectorFailFast \; \equiv \; \argmin_{\edge \in \path} \vectorp(\edge)
\end{equation}

We then show that \selectorFailFast eliminates a path optimally:
\begin{lemma}\label{lemma:fail_fast}
Given a path $\path$, \selectorFailFast minimizes the expected number of edges from $\path$ that are required to evaluated to invalidate $\path$.
\end{lemma}

\begin{proof}
Given a path $\path$, and a sequence of edges $S = \{e_1, e_2, \ldots, e_n\}$ belonging to the path,
and the corresponding priors of the edges being valid $(p_1, p_2, \ldots, p_n)$, 
let the expected number of edge evaluations to invalidate the $\path$ be $\evalEdges(S)$ which is given by
\begin{equation}
\begin{aligned}
\expect{\vectorp}{ \evalEdges(S) } &= (1-p_1) + 2 p_1 (1-p_2) + \ldots \\
&= \sum_{l=1}^{n} \left( \prod_{m=1}^{l-1} p_m \right) \left(1-p_l\right)l 
\end{aligned}
\label{eqn:greedy_expected_edge_evaluations}
\end{equation}
%Let $S$ be such that there exist two edges $e_i,~e_j \in S$ such that $p_i > p_j,~i < j$ \ie $S' = \{e_1, e_2, \ldots,e_i, \ldots, e_j, \ldots, e_n\}$. 
Without loss of generality, let $p_i > p_{i+1}$ for a given $i$. Consider the alternate sequence of evaluations $S' = \{e_1, e_2, \ldots, e_{i+1}, e_i \ldots, e_n\}$ where the positions of the edges $e_i,~e_{i+1}$ are swapped. 
%We show that by swapping the order and evaluating the edge with lower prior over probability of existence, the expected number of edge evaluations are reduced. 
Consider the difference:
\begin{equation}
\begin{aligned}
& \expect{\vectorp}{ \evalEdges(S) } - \expect{\vectorp}{ \evalEdges(S') } \\
&= \ldots + \prod_{m=1}^{i-1} p_m \left[ (1-p_i) i + p_i(1-p_{i+1})(i+1) \right] + \ldots \\
&- \ldots + \prod_{m=1}^{i-1} p_m \left[ (1-p_{i+1}) i + p_{i+1}(1-p_{i})(i+1) \right] + \ldots \\
&= \prod_{m=1}^{i-1} p_m \left[-i(p_i - p_{i+1}) + (i+1)(p_i - p_{i+1}) \right] \\
&= \prod_{m=1}^{i-1} p_m (p_i - p_{i+1}) \\
& > 0
%\left(p_i - p_j\right)\sum_{\substack{l=i-1 \\ l \neq \{i, j\}}}^{j}{\prod_{\substack{m=1 \\ m \neq \{i,j\}}}^{l}{p_m}}
\end{aligned}
\label{eqn:greedy_expected_edge_evaluations}
\end{equation}
Since each such swap results in monotonic decrease in the objective, there exists an unique fixed point, i.e., the optimal sequence $S^*$ has $p_1 \leq p_2 \leq \ldots \leq p_n$.
\end{proof}

Since each path is independent of another, each path has to be eliminated independently which \selectorFailFast does optimally.. Hence \selectorFailFast is the optimal selector. 

\section{}
\label{appendix:posterior}
We define the posterior selector in a manner similar to $\selectorFailFast$ 
\begin{equation}
	\selectorPostFailFast \; \equiv \; \argmin_{\edge \in \path} \vectorp(\edge|\state_t)
\end{equation}
where $\state_t$ is the state of search at time t. We aproximate the posterior using the training dataset of $N$ worlds similar to \citep{choudhury2017active,choudhury2018bayesian} as follows - for each training world $\world_i$ a score $z_{i}$ is calculated based on the discrepancy between $s_t$ and the $s_{ti}$ where the latter is what the state of the search would be if agent were operating in $\world_i$, i.e
\begin{equation*}
z_{i} = -|s_t - s_{ti}|
\end{equation*}  
where, the difference follows directly from defintion in \ref{sec:problem_formulation:mdp}. The probability for $\phi_i$ is then given by a softmax over training worlds,
\begin{equation*}
P(\world_i | \state_t) = \frac{e^{z_{i}}}{\sum_{\substack{k=0}}^{N} e^{z_k}}
\end{equation*}
Then, for every $\edge \in \path$,
\begin{equation}
\vectorp(\edge|\state_t) = \sum_{k=0}^{N} P(\world_k | \state_t) \world_i(\edge)
\end{equation}
